# Supplementary material for: Rectangular Rotational Invariant Estimator for General Additive Noise Matrices
Source: arXiv:2304.12264 source file (2023-04-24)
Supplement: Supplementary file 1 [file Proof-of-prop2.tex]

\subsection{Proof of proposition \ref{pseudo-lip}}\label{proof of prop2}
\begin{figure*}[t]
\centering
\begin{minipage}{\textwidth}
\begin{equation}
\begin{split}
        F_N(t) &= -\frac{1}{M N} \bE_{\bY_1^{(t)}, \bY_2^{(t)}} \bigg[ \ln \int d Q_{N,M}(\bU, \bV,  \bsig, \tilde{\bsig}) e^{N \Tr [\sqrt{\lambda t} \bX^T \bY_1^{(t)} - \frac{\lambda t}{2} \bX^T \bX +  \sqrt{\lambda (1-t)} \tilde{\bX}^T \bY_2^{(t)} - \frac{\lambda (1-t)}{2} \tilde{\bX}^T \tilde{\bX} ]} \bigg] \\
        &\hspace{-15pt}= -\frac{1}{M N} \bE_{\bY_1^{(t)}, \bY_2^{(t)}} \bigg[ \ln \int d Q_{N,M}(\bU, \bV,  \bsig, \tilde{\bsig}) e^{N \Tr [\lambda t \bX^T \bS + \sqrt{\lambda t} \bX^T \bZ_1 - \frac{\lambda t}{2} \bX^T \bX + \lambda (1-t) \tilde{\bX}^T \tilde{\bS}+  \sqrt{\lambda (1-t)} \tilde{\bX}^T \bZ_2 - \frac{\lambda (1-t)}{2} \tilde{\bX}^T \tilde{\bX}]} \bigg]
\end{split}
\label{free-energy-combined}
\end{equation}
\begin{equation}
    \frac{d}{d t}F_N(t) = -\frac{1}{M} \bE \Big[ \lambda  \Tr \langle \bX^T \bS \rangle_t + \frac{1}{2} \sqrt{\frac{\lambda}{t}} \Tr \bZ_1^T \langle \bX \rangle_t - \frac{\lambda}{2} \Tr \langle \bX^T \bX \rangle_t  - \lambda  \Tr \langle \tilde{\bX}^T \tilde{\bS} \rangle_t - \frac{1}{2} \sqrt{\frac{\lambda}{1-t}} \Tr \bZ_2^T \langle \tilde{\bX} \rangle_t + \frac{\lambda}{2} \Tr \langle \tilde{\bX}^T \tilde{\bX} \rangle_t \Big] 
    \label{time-deivative}
\end{equation}
\begin{equation}
\begin{split}
        \frac{d}{d t}F_N(t) &= -\frac{1}{M} \frac{\lambda}{2} \bE \Big[ 2 \Tr \langle \bX^T \bS \rangle_t - \Tr \langle \bX \rangle_t^T \langle \bX \rangle_t - 2 \Tr \langle \tilde{\bX}^T \tilde{\bS} \rangle_t + \Tr \langle \tilde{\bX} \rangle_t^T \langle \tilde{\bX} \rangle_t \Big] \\
        &= - \frac{1}{M} \frac{\lambda}{2} \bE \big[ \Tr [ \langle \bX^T \bS \rangle_t -  \langle \tilde{\bX}^T \tilde{\bS} \rangle_t ] \big] \hspace{10pt} \text{(By Nishimori)}
\end{split}
\label{time-deivative-Nishimori}
\end{equation}
\begin{equation}
    \begin{split}
        \frac{2 M }{\lambda} \Big|   \frac{d}{d t}F_N(t) \Big| &= \Bigg| \bE \bigg[ \Big \langle \Tr  \big[ \bS^T (\bX - \tilde{\bX})  -  (\tilde{\bS}^T - \bS)\tilde{\bX} \big] \Big\rangle_t  \bigg] \Bigg| \\
        & \leq   \bE \Bigg[ \bigg\langle \Big| \Tr  \big[ \bS^T (\bX - \tilde{\bX})  -  (\tilde{\bS}^T - \bS)\tilde{\bX} \big] \Big| \bigg\rangle_t  \Bigg] \hspace{5mm} \text{(By Jensen)} \\
        &  \leq \bE \Bigg[ \bigg\langle \Big| \Tr \bS^T (\bX - \tilde{\bX}) \Big| \bigg\rangle_t  \Bigg]   + \bE \Bigg[ \bigg\langle \Big| \Tr  (\tilde{\bS} - \bS)\tilde{\bX}^T] \Big| \bigg\rangle_t  \Bigg] \\
        & \leq    \bE \Big[ \| \bS \|_F  \langle \| \bX - \tilde{\bX} \|_F  \rangle_t  \Big]   + \bE \Big[ \| \bS - \tilde{\bS} \|_F \langle \|\tilde{\bX}\|_F \rangle_t  \Big] \\
        & \leq \sqrt{ \bE \Big[ \| \bS \|^2_F \Big] \bE \Big[ \big \langle \| \bX - \tilde{\bX} \|_F  \big \rangle_t^2  \Big] }   + \sqrt{\bE \Big[ \| \bS - \tilde{\bS} \|_F^2 \Big] \bE \Big[ \big \langle \|\tilde{\bX}\|_F \big \rangle_t^2  \Big] } \hspace{10pt} \text{(By Cauchy–Schwarz)} \\
        & \leq \sqrt{ \bE \big[ \| \bS \|^2_F \big] \bE \Big[ \big \langle \| \bX - \tilde{\bX} \|_F^2  \big \rangle_t  \Big] }   + \sqrt{\bE \big[ \| \bS - \tilde{\bS} \|_F^2 \big] \bE \Big[ \big \langle \|\tilde{\bX}\|_F^2 \big \rangle_t \Big] } \hspace{10pt} \text{(By Cauchy–Schwarz)} \\
        & = \sqrt{ \bE \big[ \| \bS \|^2_F \big] \bE \big[  \| \bS - \tilde{\bS} \|_F^2   \big] }   + \sqrt{\bE \big[ \| \bS - \tilde{\bS} \|_F^2 \big] \bE \big[ \|\tilde{\bS}\|_F^2  \big] } \hspace{10pt} \text{(By Nishimori)} \\
        &= \Big( \sqrt{ \bE \big[ \| \bS \|^2_F \big]} + \sqrt{ \bE \big[ \| \tilde{\bS} \|^2_F \big]} \Big) \sqrt{\bE \big[ \| \bS - \tilde{\bS} \|_F^2    \big]} \\
        &= \Big( \sqrt{ \bE_{\bsig} \big[ \| \bsig \|^2 \big]} + \sqrt{ \bE_{\tilde{\bsig}} \big[ \| \tilde{\bsig} \|^2 \big]} \Big) \sqrt{\bE_{\bsig, \tilde{\bsig}} \big[ \| \bsig - \tilde{\bsig} \|^2 \big] } 
    \end{split}
    \label{bounde-on-derivative}
\end{equation}
\vspace{-2mm}
\medskip
\hrule
\end{minipage}
\vspace{-5mm}
\end{figure*}

Consider two matrices with the same singular vectors, $\bS = \bU \bSig \bV^T$, $\tilde{\bS} = \bU \tilde{\bSig} \bV^T$, where $\bU \in \bR^{N \times N}, \bV \in \bR^{M \times M}$ are Haar orthogonal matrices, and $\bsig$, $\tilde{\bsig}$ are distributed according to $P_N^{(1)}(\bsig), P_N^{(2)}(\tilde{\bsig})$, respectively. For two such matrices, we write $(\bS, \tilde{\bS}) \sim Q_{N,M}(\bU, \bV,  \bsig, \tilde{\bsig})$ which is the joint p.d.f. of $\bU, \bV, \bsig, \tilde{\bsig}$,
\begin{equation*}
\begin{split}
d &Q_{N,M}(\bU, \bV,  \bsig, \tilde{\bsig}) \\
    = &d \mu_N(\bU) \, d \mu_M(\bV) \, P_N^{(1)}(\bsig) \, d \bsig \, P_N^{(2)}(\tilde{\bsig}) \, d \tilde{\blam}  
\end{split}
\end{equation*}
For $t \in [0,1]$, consider the following observation model:
\begin{equation}
    \begin{cases}
  \bY_1^{(t)} = \sqrt{\lambda t}\bS + \bZ_1\\
  \bY_2^{(t)} = \sqrt{\lambda (1-t)}\tilde{\bS} + \bZ_2
\end{cases}
\label{int-model}
\end{equation}
where $\bZ_1, \bZ_2 \in \bR^{N \times M}$ are Gaussian matrices as in \eqref{observation-matrix}, independent of each other. $(\bS, \tilde{\bS}) \sim Q_{N,M}(\bU, \bV,  \bsig, \tilde{\bsig})$. The free energy for this model can be written as \eqref{free-energy-combined}, with $\bX, \tilde{\bX}$  has the same singular vectors, $\bX = \bU \bSig \bV^T$, $\tilde{\bX} = \bU \tilde{\bSig} \bV^T$.
Note that, for $t=0$ the only term depending on $\bsig$ (in both the inner and outer expectation) is the pdf $P_N^{(1)}(\bsig)$ and we can integrate over $\bsig$ in both of the expectations, to get $F_N(0) = F_N^{(2)}(\lambda)$. Similarly, we have $F_N(1) = F_N^{(1)}(\lambda)$.

Taking the derivative w.r.t. $t$, we get \eqref{time-deivative}, where $\langle . \rangle_t$ denotes the expectation with respect to the posterior distribution of the model \eqref{int-model}. By integration by parts, we have
\begin{equation*}
\begin{split}
    \bE \big[ \Tr \bZ_1^T \langle \bX \rangle_t ] &=  \sqrt{\lambda t} \bE \Big[ \Tr \langle \bX^T \bX \rangle_t  - \Tr \langle \bX \rangle_t^T \langle \bX \rangle_t \Big]\\
    \bE \big[ \Tr \bZ_2^T \langle \tilde{\bX} \rangle_t ] &\hspace{-2pt}= \hspace{-2pt}\sqrt{\lambda (1-t)} \bE \Big[ \Tr \langle \tilde{\bX}^T \tilde{\bX} \rangle_t  - \Tr \langle \tilde{\bX} \rangle_t^T \langle \tilde{\bX} \rangle_t \Big]
\end{split}
\end{equation*}
Therefore \eqref{time-deivative} can be written as \eqref{time-deivative-Nishimori}. We obtain the result by integrating \eqref{bounde-on-derivative}, over $t$ from $0$ to $1$, and using $N \leq M$.$\hfill \square$
% \end{widetext}
