# Supplementary material for: Rectangular Rotational Invariant Estimator for General Additive Noise Matrices
Source: arXiv:2304.12264 source file (2023-04-24)
Supplement: Supplementary file 2 [file Transforms.tex]

\section{Reminder on transforms}
For a probability measure $\mu$ with support contained in$[-K, K ]$ with $K>0$, we define a generating function of (even) moments $\mathcal{M}_{\mu^2} : [0,K^{-2}] \to \bR_+$
as
\begin{equation*}
    \mathcal{M}_{\mu^2} (z) = \int \frac{1}{1-t^2 z} \, d\mu(t) - 1
\end{equation*}
\begin{remark}
Note that, for a measure $\mu$ with positive support with symmetrized measure $\bar{\mu}$, we have that $\mathcal{M}_{\mu^2} (z) = \mathcal{M}_{\bar{\mu}^2} (z)$ .
\end{remark}

For $\alpha \in [0,1]$, $T^{(\alpha)}(z) = (\alpha z +1)(z+1)$, and
\begin{equation*}
    \mathcal{H}_{\mu}^{(\alpha)}(z) = z T^{(\alpha)}\big(\mathcal{M}_{\mu^2} (z)\big)
\end{equation*}
And, the \textit{rectangular R-transform} is defined as:
\begin{equation*}
    \mathcal{C}_{\mu}^{(\alpha)}(z) = {T^{(\alpha)}}^{-1}\Big(\frac{z}{{\mathcal{H}_{\mu}^{(\alpha)}}^{-1}(z)} \Big)
\end{equation*}

For a matrix $\bA \in \bR^{N \times M}$ with $\alpha = \frac{N}{M}$ with limiting singular value distribution $\mu$, we have that:
\begin{equation*}
    \bg_{AA^T}(z) = \frac{1}{z} \Big( \mathcal{M}_{\mu^2} \big(\frac{1}{z}\big) + 1 \Big) \equiv \frac{1}{z} \Big( \mathcal{M}_{A} \big(\frac{1}{z}\big) + 1 \Big)
\end{equation*}
